# Supplementary material for: Chapter-Llama: Efficient Chaptering in Hour-Long Videos with LLMs
Source: arXiv:2504.00072 source file (2025-03-31)
Supplement: Supplementary file 1 [file qualitative1.pdf]

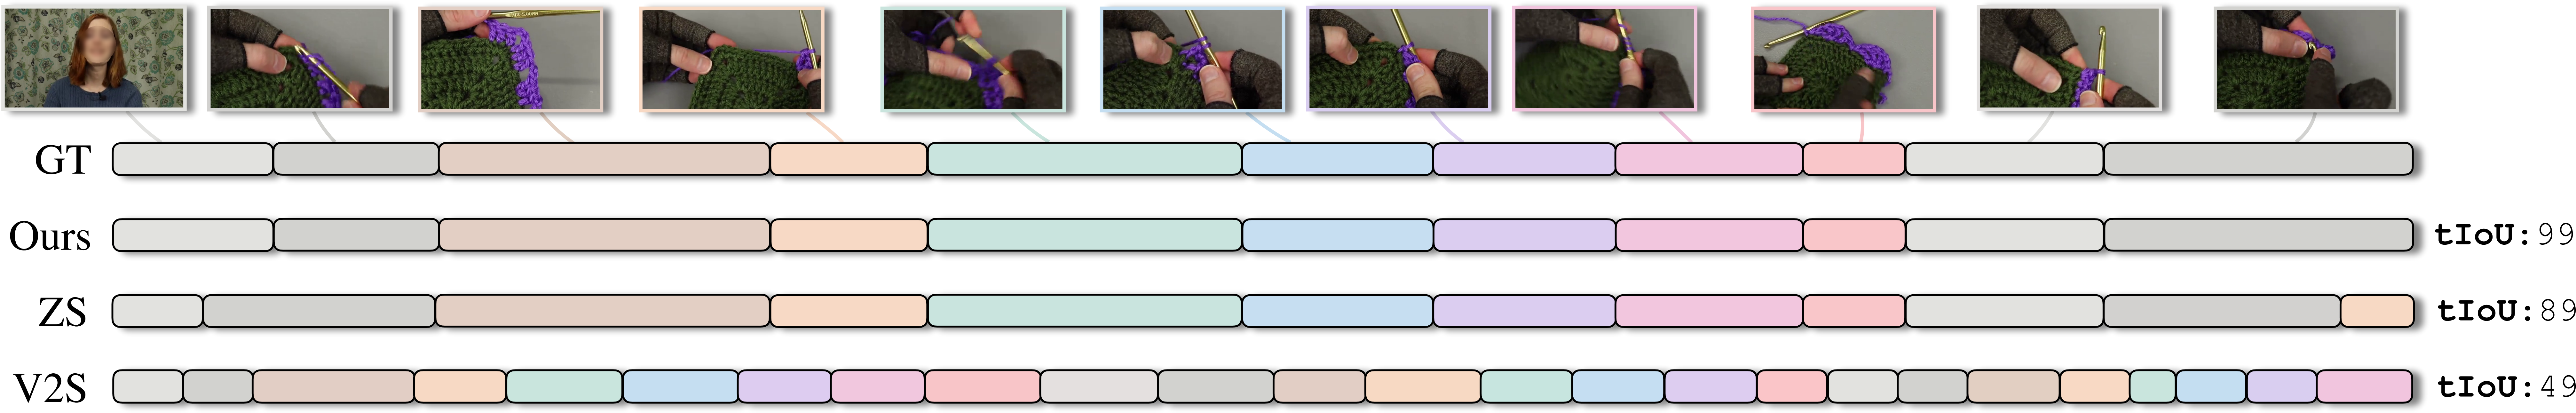


**Ground truth**
00:01:46: Double Crochet Criss Cross Border
00:03:35: Granny Square Border
00:07:13: V Stitch (Basic
00:08:56: V Stitch (Variation
00:12:23: Front Post Back Post Border
00:14:29: Treble & Chain
00:16:29: Basic Shell
00:18:32: Open Lattice Shell
00:19:39: Single Crochet Ruffle
00:21:49: Standing Ruffles

**Zero-shot:** (**S**:4, **C**:6)
00:00:00: Introduction to the video and the topic of crochet borders
00:01:00: Introduction to the materials and the first pattern, the double crochet crisscross border
00:03:33: Working the double crochet crisscross border around corners
00:07:13: Working the granny square border around corners
00:08:55: Working the basic V-stitch border around corners
00:12:22: Working the V-stitch variation border around corners
00:14:28: Working the front post back post double crochet border around corners
00:16:28: Working the treble and chain border around corners
00:18:31: Working the basic shell border around corners
00:19:38: Working the open lattice shell border around corners
00:21:48: Working the single crochet border around corners
00:24:24: Working the standing ruffle border around corners and conclusion

**Chapter-Llama** (**S**:38, **C**:296)
00:00:00: Intro
00:01:46: Double Crochet Crisscross Border
00:03:34: Granny Square Border
00:07:13: Basic V-Stitch Border
00:08:56: V-Stitch Variation Border
00:12:23: Front Post Back Post Double Crochet Border
00:14:29: Treble and Chain Border
00:16:29: Basic Shell Border
00:18:32: Open Lattice Shell Border
00:19:39: Single Crochet Border
00:21:49: Standing Ruffle Border

**Vid2Seq:** (**S**:2, **C**:8)
00:00:00: Intro.
00:00:45: Materials.
00:01:31: Double crochet crisscross border.
00:03:18: Double crochet swoop border.
00:04:19: Double crochet swoop border.
00:05:36: Double crochet swoop border.
00:06:52: Double crochet swoop border.
…
00:24:11: Outro.

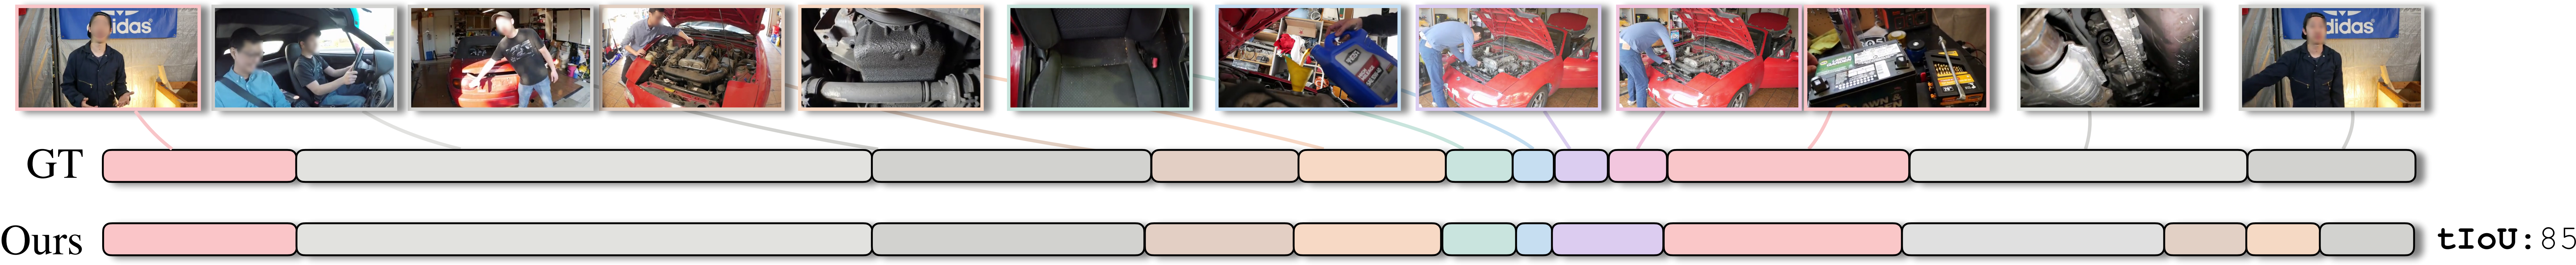


**Ground truth**

00:00:00: Car reveal
00:01:06: First drive
00:04:22: Exterior shakedown
00:05:57: Engine bay shakedown
00:06:47: Undercarriage shakedown
00:07:37: Interior shakedown
00:08:00: Maintenance begins
00:08:14: High idle / throttle body fix
00:08:32: EGR / P0470 fix
00:08:52: Lawn mower battery install
00:10:14: Driveshaft fix
00:12:09: Transmission/Diff fluid change, fuel filter, speedometer cable

**Chapter-Llama** (S:23, C:108)

00:00:00: Intro
00:01:06: First Ride
00:04:22: Exterior Walkaround
00:05:55: Engine Bay
00:06:46: Undercarriage
00:07:36: Interior
00:08:01: Oil Change
00:08:13: Throttle Body
00:08:51: Battery
00:10:12: Driveshaft
00:11:41: Test Drive
00:12:09: Transmission & Diff
00:12:34: Conclusion

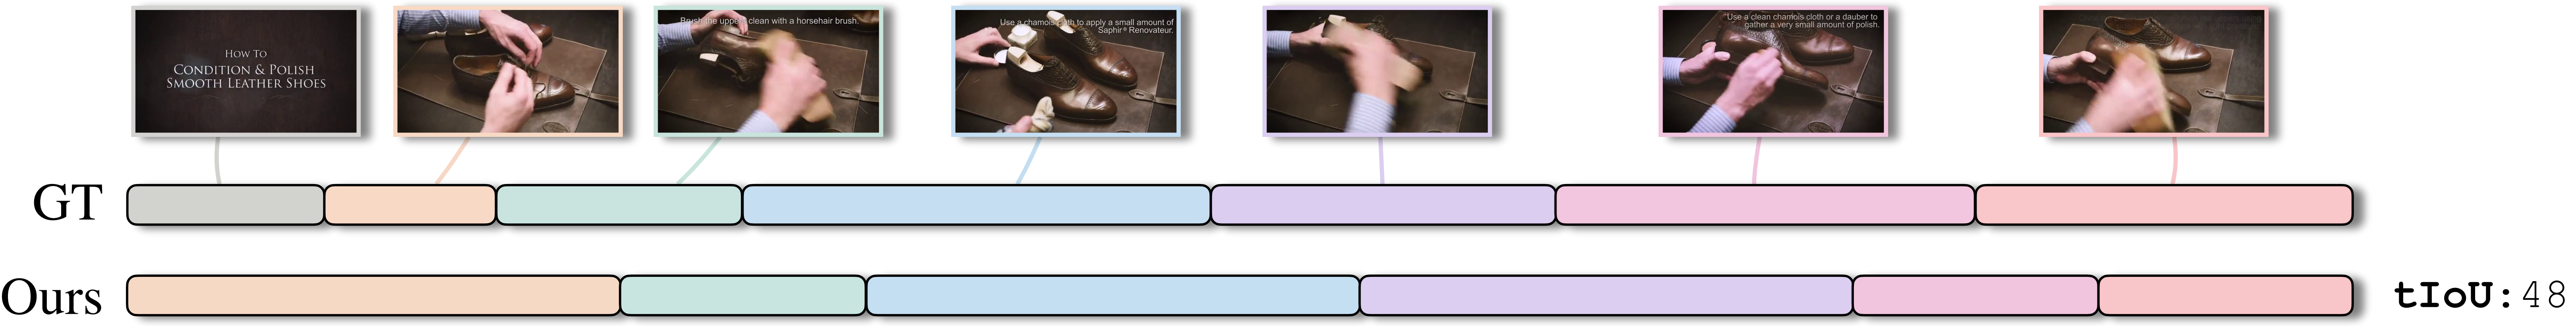


**Ground truth**
00:08: Step 1: Remove Shoelaces
00:15: Step 2: Clean
00:25: Step 3: Apply Conditioner
00:44: Step 4: Remove Excess Conditioner
00:58: Step 5: Apply Pommadier Cream Polish
01:15: Final Step: Buff with a Horsehair Brush

**Chapter-Llama** (S:3, C:8)
00:00: Remove the laces
00:20: Clean the upper part of the shoe
00:30: Apply Saphir Renovateur
00:50: Allow the product to dry
01:10: Apply pomade cream polish
01:20: Allow the cream polish to dry

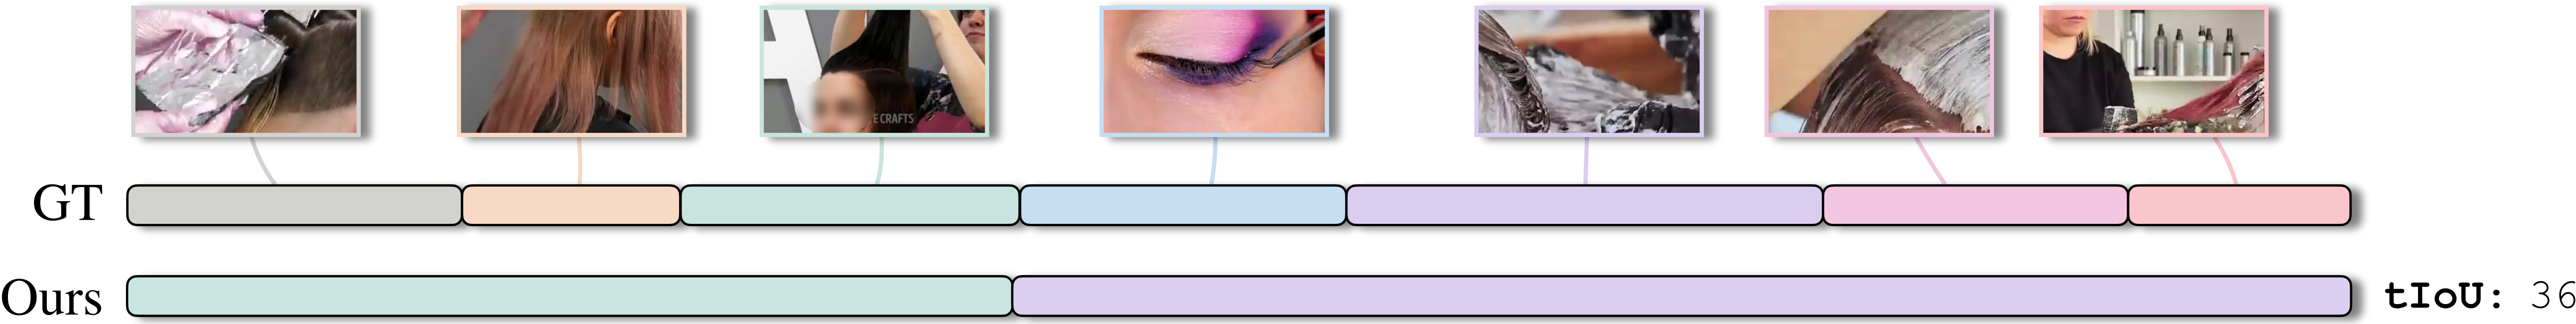


**Ground truth**
02:16: Full transformation – baby pink hair
03:45: Blonde to black hair transformation
06:03: Amazing colorful makeup tutorial
08:16: Smooth defined makeup tutorials
11:30: Black to blonde
13:34: From pink to platinum hair transformation

**Chapter-Llama:** (S:2, C:13)
00:00: Haircut
06:00: Makeup
